# Supplementary material for: Multi-Task Meta Learning: learn how to adapt to unseen tasks
Source: arXiv:2210.06989 source file (2023-04-26)
Supplement: Supplementary file 1 [file supp_matrix.tex]

\setlength{\tabcolsep}{2pt}

\begin{figure*}[ht]
\begin{center}

\begin{tabular}{c c c c c c| c c c c c}
\hline
\multirow[b]{ 2}{*}{\rotatebox[origin=t]{90}{Models}} & Input &  \multicolumn{4}{c}{\textbf{Taskonomy}} & Input & \multicolumn{4}{c}{\textbf{NYU}}\\ \cmidrule(lr){3-6} \cmidrule(lr){8-11}
% & & & & \\
& Image & Seg. & Depth & SN & Edge & Image & Seg. & Depth & SN & Edge\\
\hline
% \footnotesize{Image} &  \multicolumn{4}{c}{\adjustimage{height=1.5cm,valign=m}{images/taskonomy_mat/f8/image.jpg}} & \multicolumn{4}{c}{\adjustimage{height=1.5cm,valign=m}{images/NYU_mat/f1/image.png}}\\
% & & & & \\

% & & & & \\
\footnotesize{\rotatebox[origin=c]{90}{GT}} & \multirow[b]{ 4}{*}{\adjustimage{height=1.5cm,valign=m}{images/taskonomy_mat/f8/image.jpg}} &
\adjustimage{height=1.46cm,valign=m}{images/taskonomy_mat/f8/segmask.jpg} & \adjustimage{height=1.46cm,valign=m}{images/taskonomy_mat/f8/depthmask.jpg} & \adjustimage{height=1.46cm,valign=m}{images/taskonomy_mat/f8/surface_normal_mask.jpg} & \adjustimage{height=1.46cm,valign=m}{images/taskonomy_mat/f8/edge_mask.jpg} &
\multirow[b]{ 4}{*}{\adjustimage{height=1.5cm,valign=m}{images/NYU_mat/f1/image.png}}&
\adjustimage{height=1.5cm,valign=m}{images/NYU_mat/f1/segmask.png} & 
\adjustimage{height=1.5cm,valign=m}{images/NYU_mat/f1/depthmask.png} & \adjustimage{height=1.5cm,valign=m}{images/NYU_mat/f1/surface_normal_mask.png}& \adjustimage{height=1.5cm,valign=m}{images/NYU_mat/f1/edge_mask.png}\\
% & & & & \\
\footnotesize{\rotatebox[origin=c]{90}{Single}} & &
\adjustimage{height=1.5cm,valign=m}{images/taskonomy_mat/f8/single_seg_output.png} & \adjustimage{height=1.5cm,valign=m}{images/taskonomy_mat/f8/single_depth_output.png} & \adjustimage{height=1.5cm,valign=m}{images/taskonomy_mat/f8/single_surface_output.png} & \adjustimage{height=1.5cm,valign=m}{images/taskonomy_mat/f8/single_edge_output.png} &
&
\adjustimage{height=1.5cm,valign=m}{images/NYU_mat/f1/single_seg_output.png} & 
\adjustimage{height=1.5cm,valign=m}{images/NYU_mat/f1/single_depth_output.png} & \adjustimage{height=1.5cm,valign=m}{images/NYU_mat/f1/single_surface_output.png}& \adjustimage{height=1.5cm,valign=m}{images/NYU_mat/f1/single_edge_output.png}\\
% & & & & \\
\footnotesize{\rotatebox[origin=c]{90}{\ac{MTL}}} & &
\adjustimage{height=1.5cm,valign=m}{images/taskonomy_mat/f8/multi_seg_output.png} & \adjustimage{height=1.5cm,valign=m}{images/taskonomy_mat/f8/multi_depth_output.png} & \adjustimage{height=1.5cm,valign=m}{images/taskonomy_mat/f8/multi_surface_output.png} & \adjustimage{height=1.5cm,valign=m}{images/taskonomy_mat/f8/multi_edge_output.png} &
&
\adjustimage{height=1.5cm,valign=m}{images/NYU_mat/f1/multi_seg_output.png} & 
\adjustimage{height=1.5cm,valign=m}{images/NYU_mat/f1/multi_depth_output.png} & \adjustimage{height=1.5cm,valign=m}{images/NYU_mat/f1/multi_surface_output.png}& \adjustimage{height=1.5cm,valign=m}{images/NYU_mat/f1/multi_edge_output.png}\\
% & & & & \\
\footnotesize{\rotatebox[origin=c]{90}{\ac{MTML}}} & &
\adjustimage{height=1.5cm,valign=m}{images/taskonomy_mat/f8/seg_output.png} & \adjustimage{height=1.5cm,valign=m}{images/taskonomy_mat/f8/depth_output.png} & \adjustimage{height=1.5cm,valign=m}{images/taskonomy_mat/f8/surface_output.png} & \adjustimage{height=1.5cm,valign=m}{images/taskonomy_mat/f8/edge_output.png} &
&
\adjustimage{height=1.5cm,valign=m}{images/NYU_mat/f1/seg_output.png} & 
\adjustimage{height=1.5cm,valign=m}{images/NYU_mat/f1/depth_output.png} & \adjustimage{height=1.5cm,valign=m}{images/NYU_mat/f1/surface_output.png}& \adjustimage{height=1.5cm,valign=m}{images/NYU_mat/f1/edge_output.png}\\

\hline
\footnotesize{\rotatebox[origin=c]{90}{GT}} & \multirow[b]{ 4}{*}{\adjustimage{height=1.5cm,valign=m}{images/taskonomy_mat/f9/image.jpg}} &
\adjustimage{height=1.46cm,valign=m}{images/taskonomy_mat/f9/segmask.jpg} & \adjustimage{height=1.46cm,valign=m}{images/taskonomy_mat/f9/depthmask.jpg} & \adjustimage{height=1.46cm,valign=m}{images/taskonomy_mat/f9/surface_normal_mask.jpg} & \adjustimage{height=1.46cm,valign=m}{images/taskonomy_mat/f9/edge_mask.jpg} &
\multirow[b]{ 4}{*}{\adjustimage{height=1.5cm,valign=m}{images/NYU_mat/f2/image.png}}&
\adjustimage{height=1.5cm,valign=m}{images/NYU_mat/f2/segmask.png} & 
\adjustimage{height=1.5cm,valign=m}{images/NYU_mat/f2/depthmask.png} & \adjustimage{height=1.5cm,valign=m}{images/NYU_mat/f2/surface_normal_mask.png}& \adjustimage{height=1.5cm,valign=m}{images/NYU_mat/f2/edge_mask.png}\\
% & & & & \\
\footnotesize{\rotatebox[origin=c]{90}{Single}} & &
\adjustimage{height=1.5cm,valign=m}{images/taskonomy_mat/f9/single_seg_output.png} & \adjustimage{height=1.5cm,valign=m}{images/taskonomy_mat/f9/single_depth_output.png} & \adjustimage{height=1.5cm,valign=m}{images/taskonomy_mat/f9/single_surface_output.png} & \adjustimage{height=1.5cm,valign=m}{images/taskonomy_mat/f9/single_edge_output.png} &
&
\adjustimage{height=1.5cm,valign=m}{images/NYU_mat/f2/single_seg_output.png} & 
\adjustimage{height=1.5cm,valign=m}{images/NYU_mat/f2/single_depth_output.png} & \adjustimage{height=1.5cm,valign=m}{images/NYU_mat/f2/single_surface_output.png}& \adjustimage{height=1.5cm,valign=m}{images/NYU_mat/f2/single_edge_output.png}\\
% & & & & \\
\footnotesize{\rotatebox[origin=c]{90}{\ac{MTL}}} & &
\adjustimage{height=1.5cm,valign=m}{images/taskonomy_mat/f9/multi_seg_output.png} & \adjustimage{height=1.5cm,valign=m}{images/taskonomy_mat/f9/multi_depth_output.png} & \adjustimage{height=1.5cm,valign=m}{images/taskonomy_mat/f9/multi_surface_output.png} & \adjustimage{height=1.5cm,valign=m}{images/taskonomy_mat/f9/multi_edge_output.png} &
&
\adjustimage{height=1.5cm,valign=m}{images/NYU_mat/f2/multi_seg_output.png} & 
\adjustimage{height=1.5cm,valign=m}{images/NYU_mat/f2/multi_depth_output.png} & \adjustimage{height=1.5cm,valign=m}{images/NYU_mat/f2/multi_surface_output.png}& \adjustimage{height=1.5cm,valign=m}{images/NYU_mat/f2/multi_edge_output.png}\\
% & & & & \\
\footnotesize{\rotatebox[origin=c]{90}{\ac{MTML}}} & &
\adjustimage{height=1.5cm,valign=m}{images/taskonomy_mat/f9/seg_output.png} & \adjustimage{height=1.5cm,valign=m}{images/taskonomy_mat/f9/depth_output.png} & \adjustimage{height=1.5cm,valign=m}{images/taskonomy_mat/f9/surface_output.png} & \adjustimage{height=1.5cm,valign=m}{images/taskonomy_mat/f9/edge_output.png} &
&
\adjustimage{height=1.5cm,valign=m}{images/NYU_mat/f2/seg_output.png} & 
\adjustimage{height=1.5cm,valign=m}{images/NYU_mat/f2/depth_output.png} & \adjustimage{height=1.5cm,valign=m}{images/NYU_mat/f2/surface_output.png}& \adjustimage{height=1.5cm,valign=m}{images/NYU_mat/f2/edge_output.png}\\

\hline
\footnotesize{\rotatebox[origin=c]{90}{GT}} & \multirow[b]{ 4}{*}{\adjustimage{height=1.5cm,valign=m}{images/taskonomy_mat/f10/image.jpg}} &
\adjustimage{height=1.46cm,valign=m}{images/taskonomy_mat/f10/segmask.jpg} & \adjustimage{height=1.46cm,valign=m}{images/taskonomy_mat/f10/depthmask.jpg} & \adjustimage{height=1.46cm,valign=m}{images/taskonomy_mat/f10/surface_normal_mask.jpg} & \adjustimage{height=1.46cm,valign=m}{images/taskonomy_mat/f10/edge_mask.jpg} &
\multirow[b]{ 4}{*}{\adjustimage{height=1.5cm,valign=m}{images/NYU_mat/f3/image.png}}&
\adjustimage{height=1.5cm,valign=m}{images/NYU_mat/f3/segmask.png} & 
\adjustimage{height=1.5cm,valign=m}{images/NYU_mat/f3/depthmask.png} & \adjustimage{height=1.5cm,valign=m}{images/NYU_mat/f3/surface_normal_mask.png}& \adjustimage{height=1.5cm,valign=m}{images/NYU_mat/f3/edge_mask.png}\\
% & & & & \\
\footnotesize{\rotatebox[origin=c]{90}{Single}} & &
\adjustimage{height=1.5cm,valign=m}{images/taskonomy_mat/f10/single_seg_output.png} & \adjustimage{height=1.5cm,valign=m}{images/taskonomy_mat/f10/single_depth_output.png} & \adjustimage{height=1.5cm,valign=m}{images/taskonomy_mat/f10/single_surface_output.png} & \adjustimage{height=1.5cm,valign=m}{images/taskonomy_mat/f10/single_edge_output.png} &
&
\adjustimage{height=1.5cm,valign=m}{images/NYU_mat/f3/single_seg_output.png} & 
\adjustimage{height=1.5cm,valign=m}{images/NYU_mat/f3/single_depth_output.png} & \adjustimage{height=1.5cm,valign=m}{images/NYU_mat/f3/single_surface_output.png}& \adjustimage{height=1.5cm,valign=m}{images/NYU_mat/f3/single_edge_output.png}\\
% & & & & \\
\footnotesize{\rotatebox[origin=c]{90}{\ac{MTL}}} & &
\adjustimage{height=1.5cm,valign=m}{images/taskonomy_mat/f10/multi_seg_output.png} & \adjustimage{height=1.5cm,valign=m}{images/taskonomy_mat/f10/multi_depth_output.png} & \adjustimage{height=1.5cm,valign=m}{images/taskonomy_mat/f10/multi_surface_output.png} & \adjustimage{height=1.5cm,valign=m}{images/taskonomy_mat/f10/multi_edge_output.png} &
&
\adjustimage{height=1.5cm,valign=m}{images/NYU_mat/f3/multi_seg_output.png} & 
\adjustimage{height=1.5cm,valign=m}{images/NYU_mat/f3/multi_depth_output.png} & \adjustimage{height=1.5cm,valign=m}{images/NYU_mat/f3/multi_surface_output.png}& \adjustimage{height=1.5cm,valign=m}{images/NYU_mat/f3/multi_edge_output.png}\\
% & & & & \\
\footnotesize{\rotatebox[origin=c]{90}{\ac{MTML}}} & &
\adjustimage{height=1.5cm,valign=m}{images/taskonomy_mat/f10/seg_output.png} & \adjustimage{height=1.5cm,valign=m}{images/taskonomy_mat/f10/depth_output.png} & \adjustimage{height=1.5cm,valign=m}{images/taskonomy_mat/f10/surface_output.png} & \adjustimage{height=1.5cm,valign=m}{images/taskonomy_mat/f10/edge_output.png} &
&
\adjustimage{height=1.5cm,valign=m}{images/NYU_mat/f3/seg_output.png} & 
\adjustimage{height=1.5cm,valign=m}{images/NYU_mat/f3/depth_output.png} & \adjustimage{height=1.5cm,valign=m}{images/NYU_mat/f3/surface_output.png}& \adjustimage{height=1.5cm,valign=m}{images/NYU_mat/f3/edge_output.png}\\

% % & & & & \\

\end{tabular}
    
\end{center}
% \vspace{-0.45cm}
% \caption{The figure illustrates sample images of the input, its corresponding ground truths, single task (Exp. 1), \ac{MTL} (Exp. 2.3) and \ac{MTML} (Exp. 5.4) outputs for semantic segmentation (Seg.), depth estimation (Depth), surface normal estimation (SN), and edge detection (Edge) for both the NYU-v2 and taskonomy_mat datasets. Note: single-task models were trained individually for all tasks, while \ac{MTL} and \ac{MTML} used a multi-task network architecture.} 

\label{fig:img_mat_1}
\end{figure*}

\setlength{\tabcolsep}{2pt}

\begin{figure*}[ht]
\begin{center}

\begin{tabular}{c c c c c c| c c c c c}
\hline
\multirow[b]{ 2}{*}{\rotatebox[origin=t]{90}{Models}} & Input &  \multicolumn{4}{c}{\textbf{Taskonomy}} & Input & \multicolumn{4}{c}{\textbf{NYU}}\\ \cmidrule(lr){3-6} \cmidrule(lr){8-11}
% & & & & \\
& Image & Seg. & Depth & SN & Edge & Image & Seg. & Depth & SN & Edge\\
\hline
% \footnotesize{Image} &  \multicolumn{4}{c}{\adjustimage{height=1.5cm,valign=m}{images/taskonomy_mat/f8/image.jpg}} & \multicolumn{4}{c}{\adjustimage{height=1.5cm,valign=m}{images/NYU_mat/f1/image.png}}\\
% & & & & \\
\footnotesize{\rotatebox[origin=c]{90}{GT}} & \multirow[b]{ 4}{*}{\adjustimage{height=1.5cm,valign=m}{images/taskonomy_mat/f15/image.jpg}} &
\adjustimage{height=1.46cm,valign=m}{images/taskonomy_mat/f15/segmask.jpg} & \adjustimage{height=1.46cm,valign=m}{images/taskonomy_mat/f15/depthmask.jpg} & \adjustimage{height=1.46cm,valign=m}{images/taskonomy_mat/f15/surface_normal_mask.jpg} & \adjustimage{height=1.46cm,valign=m}{images/taskonomy_mat/f15/edge_mask.jpg} &
\multirow[b]{ 4}{*}{\adjustimage{height=1.5cm,valign=m}{images/NYU_mat/f9/image.png}}&
\adjustimage{height=1.5cm,valign=m}{images/NYU_mat/f9/segmask.png} & 
\adjustimage{height=1.5cm,valign=m}{images/NYU_mat/f9/depthmask.png} & \adjustimage{height=1.5cm,valign=m}{images/NYU_mat/f9/surface_normal_mask.png}& \adjustimage{height=1.5cm,valign=m}{images/NYU_mat/f9/edge_mask.png}\\
% & & & & \\
\footnotesize{\rotatebox[origin=c]{90}{Single}} & &
\adjustimage{height=1.5cm,valign=m}{images/taskonomy_mat/f15/single_seg_output.png} & \adjustimage{height=1.5cm,valign=m}{images/taskonomy_mat/f15/single_depth_output.png} & \adjustimage{height=1.5cm,valign=m}{images/taskonomy_mat/f15/single_surface_output.png} & \adjustimage{height=1.5cm,valign=m}{images/taskonomy_mat/f15/single_edge_output.png} &
&
\adjustimage{height=1.5cm,valign=m}{images/NYU_mat/f9/single_seg_output.png} & 
\adjustimage{height=1.5cm,valign=m}{images/NYU_mat/f9/single_depth_output.png} & \adjustimage{height=1.5cm,valign=m}{images/NYU_mat/f9/single_surface_output.png}& \adjustimage{height=1.5cm,valign=m}{images/NYU_mat/f9/single_edge_output.png}\\
% & & & & \\
\footnotesize{\rotatebox[origin=c]{90}{\ac{MTL}}} & &
\adjustimage{height=1.5cm,valign=m}{images/taskonomy_mat/f15/multi_seg_output.png} & \adjustimage{height=1.5cm,valign=m}{images/taskonomy_mat/f15/multi_depth_output.png} & \adjustimage{height=1.5cm,valign=m}{images/taskonomy_mat/f15/multi_surface_output.png} & \adjustimage{height=1.5cm,valign=m}{images/taskonomy_mat/f15/multi_edge_output.png} &
&
\adjustimage{height=1.5cm,valign=m}{images/NYU_mat/f9/multi_seg_output.png} & 
\adjustimage{height=1.5cm,valign=m}{images/NYU_mat/f9/multi_depth_output.png} & \adjustimage{height=1.5cm,valign=m}{images/NYU_mat/f9/multi_surface_output.png}& \adjustimage{height=1.5cm,valign=m}{images/NYU_mat/f9/multi_edge_output.png}\\
% & & & & \\
\footnotesize{\rotatebox[origin=c]{90}{\ac{MTML}}} & &
\adjustimage{height=1.5cm,valign=m}{images/taskonomy_mat/f15/seg_output.png} & \adjustimage{height=1.5cm,valign=m}{images/taskonomy_mat/f15/depth_output.png} & \adjustimage{height=1.5cm,valign=m}{images/taskonomy_mat/f15/surface_output.png} & \adjustimage{height=1.5cm,valign=m}{images/taskonomy_mat/f15/edge_output.png} &
&
\adjustimage{height=1.5cm,valign=m}{images/NYU_mat/f9/seg_output.png} & 
\adjustimage{height=1.5cm,valign=m}{images/NYU_mat/f9/depth_output.png} & \adjustimage{height=1.5cm,valign=m}{images/NYU_mat/f9/surface_output.png}& \adjustimage{height=1.5cm,valign=m}{images/NYU_mat/f9/edge_output.png}\\

\hline

\footnotesize{\rotatebox[origin=c]{90}{GT}} & \multirow[b]{ 4}{*}{\adjustimage{height=1.5cm,valign=m}{images/taskonomy_mat/f16/image.jpg}} &
\adjustimage{height=1.46cm,valign=m}{images/taskonomy_mat/f16/segmask.jpg} & \adjustimage{height=1.46cm,valign=m}{images/taskonomy_mat/f16/depthmask.jpg} & \adjustimage{height=1.46cm,valign=m}{images/taskonomy_mat/f16/surface_normal_mask.jpg} & \adjustimage{height=1.46cm,valign=m}{images/taskonomy_mat/f16/edge_mask.jpg} &
\multirow[b]{ 4}{*}{\adjustimage{height=1.5cm,valign=m}{images/NYU_mat/f6/image.png}}&
\adjustimage{height=1.5cm,valign=m}{images/NYU_mat/f6/segmask.png} & 
\adjustimage{height=1.5cm,valign=m}{images/NYU_mat/f6/depthmask.png} & \adjustimage{height=1.5cm,valign=m}{images/NYU_mat/f6/surface_normal_mask.png}& \adjustimage{height=1.5cm,valign=m}{images/NYU_mat/f6/edge_mask.png}\\
% & & & & \\
\footnotesize{\rotatebox[origin=c]{90}{Single}} & &
\adjustimage{height=1.5cm,valign=m}{images/taskonomy_mat/f16/single_seg_output.png} & \adjustimage{height=1.5cm,valign=m}{images/taskonomy_mat/f16/single_depth_output.png} & \adjustimage{height=1.5cm,valign=m}{images/taskonomy_mat/f16/single_surface_output.png} & \adjustimage{height=1.5cm,valign=m}{images/taskonomy_mat/f16/single_edge_output.png} &
&
\adjustimage{height=1.5cm,valign=m}{images/NYU_mat/f6/single_seg_output.png} & 
\adjustimage{height=1.5cm,valign=m}{images/NYU_mat/f6/single_depth_output.png} & \adjustimage{height=1.5cm,valign=m}{images/NYU_mat/f6/single_surface_output.png}& \adjustimage{height=1.5cm,valign=m}{images/NYU_mat/f6/single_edge_output.png}\\
% & & & & \\
\footnotesize{\rotatebox[origin=c]{90}{\ac{MTL}}} & &
\adjustimage{height=1.5cm,valign=m}{images/taskonomy_mat/f16/multi_seg_output.png} & \adjustimage{height=1.5cm,valign=m}{images/taskonomy_mat/f16/multi_depth_output.png} & \adjustimage{height=1.5cm,valign=m}{images/taskonomy_mat/f16/multi_surface_output.png} & \adjustimage{height=1.5cm,valign=m}{images/taskonomy_mat/f16/multi_edge_output.png} &
&
\adjustimage{height=1.5cm,valign=m}{images/NYU_mat/f6/multi_seg_output.png} & 
\adjustimage{height=1.5cm,valign=m}{images/NYU_mat/f6/multi_depth_output.png} & \adjustimage{height=1.5cm,valign=m}{images/NYU_mat/f6/multi_surface_output.png}& \adjustimage{height=1.5cm,valign=m}{images/NYU_mat/f6/multi_edge_output.png}\\
% & & & & \\
\footnotesize{\rotatebox[origin=c]{90}{\ac{MTML}}} & &
\adjustimage{height=1.5cm,valign=m}{images/taskonomy_mat/f16/seg_output.png} & \adjustimage{height=1.5cm,valign=m}{images/taskonomy_mat/f16/depth_output.png} & \adjustimage{height=1.5cm,valign=m}{images/taskonomy_mat/f16/surface_output.png} & \adjustimage{height=1.5cm,valign=m}{images/taskonomy_mat/f16/edge_output.png} &
&
\adjustimage{height=1.5cm,valign=m}{images/NYU_mat/f6/seg_output.png} & 
\adjustimage{height=1.5cm,valign=m}{images/NYU_mat/f6/depth_output.png} & \adjustimage{height=1.5cm,valign=m}{images/NYU_mat/f6/surface_output.png}& \adjustimage{height=1.5cm,valign=m}{images/NYU_mat/f6/edge_output.png}\\

\hline
\footnotesize{\rotatebox[origin=c]{90}{GT}} & \multirow[b]{ 4}{*}{\adjustimage{height=1.5cm,valign=m}{images/taskonomy_mat/f17/image.jpg}} &
\adjustimage{height=1.46cm,valign=m}{images/taskonomy_mat/f17/segmask.jpg} & \adjustimage{height=1.46cm,valign=m}{images/taskonomy_mat/f17/depthmask.jpg} & \adjustimage{height=1.46cm,valign=m}{images/taskonomy_mat/f17/surface_normal_mask.jpg} & \adjustimage{height=1.46cm,valign=m}{images/taskonomy_mat/f17/edge_mask.jpg} &
\multirow[b]{ 4}{*}{\adjustimage{height=1.5cm,valign=m}{images/NYU_mat/f8/image.png}}&
\adjustimage{height=1.5cm,valign=m}{images/NYU_mat/f8/segmask.png} & 
\adjustimage{height=1.5cm,valign=m}{images/NYU_mat/f8/depthmask.png} & \adjustimage{height=1.5cm,valign=m}{images/NYU_mat/f8/surface_normal_mask.png}& \adjustimage{height=1.5cm,valign=m}{images/NYU_mat/f8/edge_mask.png}\\
% & & & & \\
\footnotesize{\rotatebox[origin=c]{90}{Single}} & &
\adjustimage{height=1.5cm,valign=m}{images/taskonomy_mat/f17/single_seg_output.png} & \adjustimage{height=1.5cm,valign=m}{images/taskonomy_mat/f17/single_depth_output.png} & \adjustimage{height=1.5cm,valign=m}{images/taskonomy_mat/f17/single_surface_output.png} & \adjustimage{height=1.5cm,valign=m}{images/taskonomy_mat/f17/single_edge_output.png} &
&
\adjustimage{height=1.5cm,valign=m}{images/NYU_mat/f8/single_seg_output.png} & 
\adjustimage{height=1.5cm,valign=m}{images/NYU_mat/f8/single_depth_output.png} & \adjustimage{height=1.5cm,valign=m}{images/NYU_mat/f8/single_surface_output.png}& \adjustimage{height=1.5cm,valign=m}{images/NYU_mat/f8/single_edge_output.png}\\
% & & & & \\
\footnotesize{\rotatebox[origin=c]{90}{\ac{MTL}}} & &
\adjustimage{height=1.5cm,valign=m}{images/taskonomy_mat/f17/multi_seg_output.png} & \adjustimage{height=1.5cm,valign=m}{images/taskonomy_mat/f17/multi_depth_output.png} & \adjustimage{height=1.5cm,valign=m}{images/taskonomy_mat/f17/multi_surface_output.png} & \adjustimage{height=1.5cm,valign=m}{images/taskonomy_mat/f17/multi_edge_output.png} &
&
\adjustimage{height=1.5cm,valign=m}{images/NYU_mat/f8/multi_seg_output.png} & 
\adjustimage{height=1.5cm,valign=m}{images/NYU_mat/f8/multi_depth_output.png} & \adjustimage{height=1.5cm,valign=m}{images/NYU_mat/f8/multi_surface_output.png}& \adjustimage{height=1.5cm,valign=m}{images/NYU_mat/f8/multi_edge_output.png}\\
% & & & & \\
\footnotesize{\rotatebox[origin=c]{90}{\ac{MTML}}} & &
\adjustimage{height=1.5cm,valign=m}{images/taskonomy_mat/f17/seg_output.png} & \adjustimage{height=1.5cm,valign=m}{images/taskonomy_mat/f17/depth_output.png} & \adjustimage{height=1.5cm,valign=m}{images/taskonomy_mat/f17/surface_output.png} & \adjustimage{height=1.5cm,valign=m}{images/taskonomy_mat/f17/edge_output.png} &
&
\adjustimage{height=1.5cm,valign=m}{images/NYU_mat/f8/seg_output.png} & 
\adjustimage{height=1.5cm,valign=m}{images/NYU_mat/f8/depth_output.png} & \adjustimage{height=1.5cm,valign=m}{images/NYU_mat/f8/surface_output.png}& \adjustimage{height=1.5cm,valign=m}{images/NYU_mat/f8/edge_output.png}\\

\end{tabular}
    
\end{center}
% \vspace{-0.45cm}
\caption{The figure illustrates images of the input, its corresponding ground truths, single task (Exp. 1), \ac{MTL} (Exp. 2.3) and \ac{MTML} (Exp. 5.4) outputs for semantic segmentation (Seg.), depth estimation (Depth), surface normal estimation (SN), and edge detection (Edge) for both the NYU-v2 and taskonomy datasets. Note: single-task models were trained individually for all tasks, while \ac{MTL} and \ac{MTML} used a multi-task network architecture.} 

\label{fig:img_mat_supp}
\end{figure*}
